# Supplementary material for: XRay: Enhancing the Web's Transparency with Differential Correlation
Source: arXiv:1407.2323 source file (2014-10-07)
Supplement: Supplementary file 1 [file implementation-appendix.tex]

\section{Implementation Details}
\label{s:implementation_details}

\subsection{Automatic Gmail Account Creation}
\label{s:twilio}
We automated the creation of shadow accounts.
Creating Amazon accounts was not difficult because it only required an email
address.
Creating Gmail accounts, on the other hand, is trickier because Google tries
to stop automated account creation more aggressively than Amazon.
To appear less suspicious to Google, we verified accounts using phone numbers
bought and managed using Twilio.
Gmail blocks Twilio numbers by default so we used the Twilio numbers to
instantiate Google Voice accounts which are allowed by Gmail.
Using Google Voice Leverage we created three Google Voice accounts per Twilio
number, by automatically answering phone calls and inputting verification codes.
Each Voice number allowed for five Gmail accounts verifications, leading to
fifteen Gmail accounts per Twilio number.
With this technique, we created more than 500 Google accounts for
less than 0.07\$ a piece. It seems that Google is more aggressive in
blocking Google Voice Leverage now, making account creation more expansive.
 
\subsection{Performance Evaluation}
\label{s:eval:performance}
We evaluate performances on two main components: the user facing block and the 
backend. First, the user facing component consists in the chrome plugin and an
API exposed by \xray.  The API returns the associations found for an ad passed
as argument.  Queries run in real time (a few dozen milliseconds).  This is
important for usability: the user can see visual feedback on targeting while
browsing.  The chrome plugin makes requests in the background and displays
results when data is available.  The overhead when browsing Gmail is less than
0.3\%, which doesn't affect user experience.
Second, the backend block runs asynchronously; it populates and scrap the shadow
accounts, and performs data analysis every few hours. We didn't spend any time
optimizing this process as it doesn't degrade user experience, but it is highly
parallelizable.
